# Supplementary material for: Mitigating Dataset Bias by Using Per-sample Gradient
Source: arXiv:2205.15704 source file (2023-02-10)
Supplement: Supplementary file 1 [file exp_neurips.tex]

\section{Experiment details \revision{and additional analysis}} 
\label{app:exp}

\subsection{Settings}
\label{app:exp_setting}

\myparagraph{Architecture.}
For the colored MNIST, and Multi-Bias MNIST datasets, we use simple convolutional networks consisting of three CNN layers with kernel size 4, and channel size \{8, 32, 64\} for each layer. Also, we utilize average pooling at the end of each layer. Batch normalization and dropout techniques are used for regularization. Detailed network configurations are below. For corrupted CIFAR, BAR, and BFFHQ, we utilize ResNet-18 which is provided by the open source library, \code{torchvision}.

\myparagraph{SimConv-1.}

\code{(conv1): Conv2d(3, 8, kernel\_size=(4, 4), stride=(1, 1))\\
(bn1): BatchNorm2d(8, eps=1e-05, momentum=0.1, affine=True, track\_running\_stats=True)\\
(relu1): ReLU()\\
(dropout1): Dropout(p=0.5, inplace=False)\\
(avgpool1): AvgPool2d(kernel\_size=2, stride=2, padding=0)\\
(conv2): Conv2d(8, 32, kernel\_size=(4, 4), stride=(1, 1))\\
(bn2): BatchNorm2d(32, eps=1e-05, momentum=0.1, affine=True, track\_running\_stats=True)\\
(relu2): ReLU()\\
(dropout2): Dropout(p=0.5, inplace=False)\\
(avgpool2): AvgPool2d(kernel\_size=2, stride=2, padding=0)\\
(conv3): Conv2d(32, 64, kernel\_size=(4, 4), stride=(1, 1))\\
(relu3): ReLU()\\
(bn3): BatchNorm2d(64, eps=1e-05, momentum=0.1, affine=True, track\_running\_stats=True)\\
(dropout3): Dropout(p=0.5, inplace=False)\\
(avgpool3): AdaptiveAvgPool2d(output\_size=(1, 1))\\
(fc): Linear(in\_features=64, out\_features=\textbf{\$num\_class}, bias=True)
}

\myparagraph{SimConv-2.}

\code{(conv1): Conv2d(3, 8, kernel\_size=(7, 7), stride=(1, 1))\\
(bn1): BatchNorm2d(8, eps=1e-05, momentum=0.1, affine=True, track\_running\_stats=True)\\
(relu1): ReLU()\\
(dropout1): Dropout(p=0.5, inplace=False)\\
(avgpool1): AvgPool2d(kernel\_size=3, stride=3, padding=0)\\
(conv2): Conv2d(8, 32, kernel\_size=(7, 7), stride=(1, 1))\\
(bn2): BatchNorm2d(32, eps=1e-05, momentum=0.1, affine=True, track\_running\_stats=True)\\
(relu2): ReLU()\\
(dropout2): Dropout(p=0.5, inplace=False)\\
(avgpool2): AvgPool2d(kernel\_size=3, stride=3, padding=0)\\
(conv3): Conv2d(32, 64, kernel\_size=(5, 5), stride=(1, 1))\\
(relu3): ReLU()\\
(bn3): BatchNorm2d(64, eps=1e-05, momentum=0.1, affine=True, track\_running\_stats=True)\\
(dropout3): Dropout(p=0.5, inplace=False)\\
(conv4): Conv2d(64, 128, kernel\_size=(3, 3), stride=(1, 1))\\
(relu4): ReLU()\\
(bn4): BatchNorm2d(128, eps=1e-05, momentum=0.1, affine=True, track\_running\_stats=True)\\
(dropout4): Dropout(p=0.5, inplace=False)\\
(avgpool): AdaptiveAvgPool2d(output\_size=(1, 1))\\
(fc): Linear(in\_features=128, out\_features=\textbf{\$num\_class}, bias=True)}

\subsection{Baselines}

\label{app:exp_baseline}
(1) ReBias~\cite{bahng2019learning} attempts to mitigate texture bias utilizing the Hilbert-Schmidt Independence Criterion. For fair comparison, we utilize the same networks for biased model and debiased model, while in the original implementation, the authors utilized BagNet which captures local information by reducing the size of kernel of convolutional layers. Loss function that this work proposed are as follows. Details are in the original paper.
\begin{equation*}
    \min_{f \in F} \left\{ \mc{L}(f,X,Y) + \lambda \max_{g \in G} \text{HSIC}_1(f,g) \right\}.
\end{equation*}
Here, $f$ and $g$ are biased and debiased models, respectively. $\text{HSIC}_1$ is Hilbert-Schmidt independence criterion.

(2) LfF~\cite{nam2020learning} trains the debiased model by weighting the bias-conflicting samples based on the ``relative difficulty'' which is computed by the two loss values from the biased model and debiased model. To emphasize bias-conflict samples, the authors utilize generalized cross entropy loss with parameter $\alpha=0.7$. We implement the LfF algorithm following the official code offered by the authors. Loss function that this work proposed are as follows. Details are in the original paper.
\begin{align*}
    \mc{L}_\text{LfF} &= W(z) \mc{L}_{\text{CE}} (C_d(z, y) + \lambda \mc{L}_{\text{GCE}} (C_b(z,y)),\\
    W(z)  &= \frac{\mc{L}_{\text{CE}}(C_b(z) , y)}{\mc{L}_{\text{CE}}(C_b(z),y) + \mc{L}_{\text{CE}}(C_d(z), y)}.
\end{align*}
Note that $W(z)$ is a relative difficulty and that GCE is a generalized cross-entorpy. $z$ denotes feature, which is the output of the penultimate layer, and $C_{\cdot}$ is fully connected layer. 

(3) JTT~\cite{liu2021just} aims to debiasing by spliting dataset into correctly learned and failed to learned samples. To do so, JTT trains the biased model first and split the given training dataset as follows:
    \begin{equation}
        \mc{D}_\text{error-set} = \{(x, y) \text{ s.t. } y_\text{given} \neq  \argmax_c f_b(x)[c] \},
    \end{equation}
    Then, train the ultimate debiased model by oversampling $\mc{D}_\text{error-set}$ with $\lambda_{up}$ times. We set $\lambda_{up}$ as $1./\rho$ for all experiments. We reproduce the results by utilizing the official code offered by the authors. The main strength of PGD compared to JTT is that PGD does not need to set a hyperparameter. 

(4) Disen~\cite{lee2021learning} aims to debias by generating abundant features from mixing features between samples. To do so, the authorus train the biased and debiased model by aggregating features from both networks. This work also utilized ``relative difficulty'' that is proposed in LfF~\cite{nam2020learning}. We reproduce the results utilizing the official code offered by the authors. The loss function proposed in this work is as follows. Details are provided in the original paper.
\begin{equation*}
    \mc{L}_\text{total} = \mc{L}_\text{dis} + \lambda_\text{swap}\mc{L}_\text{swap},
\end{equation*}
where 
\begin{align*}
    \mc{L}_\text{swap} &= W(z) \mc{L}_{\text{CE}} (C_d(z_\text{swap}, y) + \lambda_{\text{swap}_b} \mc{L}_{\text{GCE}} (C_b(z_\text{swap},\tilde{y})) \\
    \mc{L}_\text{dis} &= W(z) \mc{L}_{\text{CE}} (C_d(z, y) + \lambda_{\text{dis}} \mc{L}_{\text{GCE}} (C_b(z,y)),\\
    W(z)  &= \frac{\mc{L}_{\text{CE}}(C_b(z) , y)}{\mc{L}_{\text{CE}}(C_b(z),y) + \mc{L}_{\text{CE}}(C_d(z), y)}.
\end{align*}
All terms are identical with LfF paper, except for swapped feature $z_\text{swap}$.

\subsection{Implementation Details}

\myparagraph{Image processing}
We train and evaluate with a fixed image size. For colored MNIST  case, $28\times 28$ and Multi-bias MNIST , $56\times 56$, Corrupted CIFAR, $32\times 32$, and real-world datasets of $224\times224$. For all cases, we utilize random rotation and color jitter to avoid overfitting. We use normalizing with mean $0.4914, 0.4822, 0.4465)$, and standard deviation $(0.2023, 0.1994, 0.2010)$.

\myparagraph{Implementation}
For all tables reported in Section~\ref{sec:exp}, we reproduce all experimental results referring to other official repositories:
\footnote{https://github.com/alinlab/LfF}
\footnote{https://github.com/clovaai/rebias}
\footnote{https://github.com/kakaoenterprise/Learning-Debiased-Disentangled}
\footnote{https://github.com/anniesch/jtt}.

Except for JTT, all hyperparameters for corrupted CIFAR, BAR, and BFFHQ follow previously reported parameters in repositories. We grid-search for other cases, MNIST variants. We set the only hyperparameter of PGD, q, as 0.7, which is proposed by the original paper~\cite{zhang2018generalized}. A summary of the hyperparameters that we used is reported in Table~\ref{tab:hyperparam}. We conduct our experiments mainly using a single Titan XP GPU for all cases.

\begin{table}[h]
    \centering
    \resizebox{0.9\textwidth}{!}{
        \begin{tabular}{c|c|c|c|c|c}
            \thickhline
              & Colored MNIST & Multi-bias MNIST & Corrupted CIFAR & BAR & Biased FFHQ \\
              \hline
Optimizer     & SGD           & SGD              & Adam            & SGD                       & Adam        \\
Batch size    & 128           & 32               & 256             & 16                        & 64          \\
Learning rate & 0.02          & 0.01             & 0.001           & 0.0005                    & 0.0001      \\
Weight decay  & 0.001         & 0.0001           & 0.001           & 1e-5                      & 0.000      \\
Momentum      & 0.9           & 0.9              & -               & 0.9                       & -           \\
Lr decay      & 0.1           & 0.1              & 0.5             & 0.1                       & 0.1         \\
Decay step    & 40            & -                & 40              & 20                        & 32          \\
Epoch         & 100           & 100              & 200             & 100                       & 160  \\
GCE $\alpha$  & 0.7           & 0.7              & 0.7             & 0.7                       & 0.7  \\
        \thickhline
\end{tabular}}
\caption{Hyperparameter details}
\label{tab:hyperparam}
\end{table}

\begin{wraptable}[7]{r}{0.4\textwidth}
    \vspace{0.2in}
    \centering
    \resizebox{0.4\textwidth}{!}{
    \begin{tabular}{ccc|cc}
            \thickhline
                            & \multicolumn{2}{c}{CelebA}        & \multicolumn{2}{c}{Waterbird}        \\
            Algorithm       & Avg    & Worst        & Avg & Worst\\ \hline
            Vanilla$^\dagger$          & 95.7  &  47.2   & 94.6  & 93.1    \\ 
            EIIL$^\ddagger$          & -  &  -   & 96.9  & 78.7    \\ 
            George$^\dagger$        & 94.6  &  53.7  & 95.7  & 76.2    \\ 
            Ours                    & 93.1  &  \textbf{54.4}   & 96.7  & \textbf{79.3}    \\ 
            \thickhline
    \end{tabular}
    }
    \caption{CelebA and Waterbird dataset. $\dagger$ and $\ddagger$ mark the performance reported by~\cite{sohoni2020no} and~\cite{creager2021environment}. }
    \label{tab:celeb_waterbird}
\end{wraptable}

\subsection{Additional experiments}

\revision{\subsubsection{CelebA~\cite{liu2015faceattributes} and Waterbird~\cite{sagawa2019distributionally} dataset}
For further analysis, we examine two real-world datasets, CelebA~\cite{liu2015faceattributes} and Waterbird~\cite{sagawa2019distributionally}. These benchmarks are tested in~\cite{nam2020learning, creager2021environment, sohoni2020no}. The PGD results are given in Table~\ref{tab:celeb_waterbird}. The worst group performance, which is used as the main metric in previous work~\cite{nam2020learning, creager2021environment, sohoni2020no}, is superior to other algorithms. This result represents that PGD works real-world applications.  }

% We present additional findings derived from two real-world datasets, CelebA and Waterbird, for further examination. These benchmarks consists of datasets used in ~\cite{nam2020learning, creager2021environment, sohoni2020no}. In Table~\ref{tab:celeb_waterbird}, the experimental results of PGD are described. Note that we adhere to the same experimental parameters~\cite{nam2020learning, creager2021environment, sohoni2020no}. As shown in Table~\ref{tab:celeb_waterbird}, the worst group performance, which is the main comparison metric of other papers~\cite{sagawa2019distributionally, creager2021environment, sohoni2020no}, outperforms other algorithms.}

\begin{figure*}[h]
    \centering
    \subfloat[Colored MNIST $\rho=0.5\%$]{\includegraphics[width=0.32\textwidth]{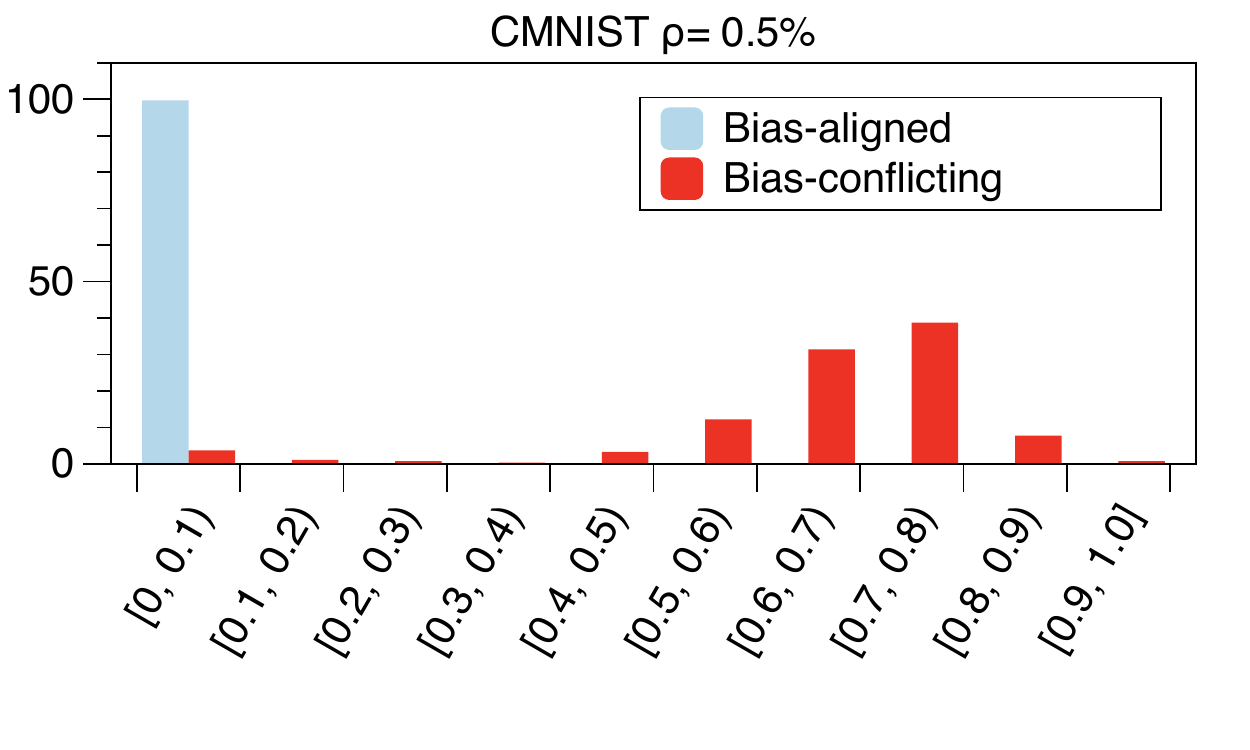} \label{fig:hist_0.5}}
    \subfloat[Colored MNIST $\rho=1\%$]{\includegraphics[width=0.32\textwidth]{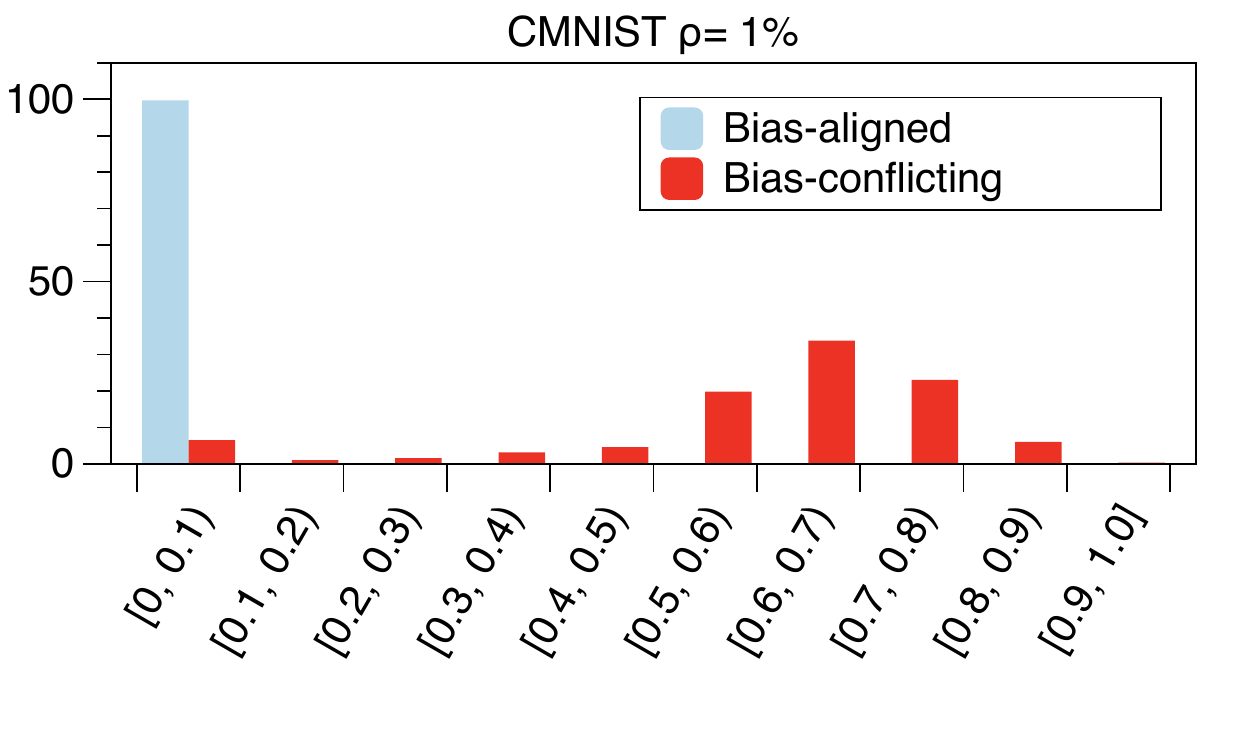} \label{fig:hist_1}}
    \subfloat[Colored MNIST $\rho=5\%$]{\includegraphics[width=0.32\textwidth]{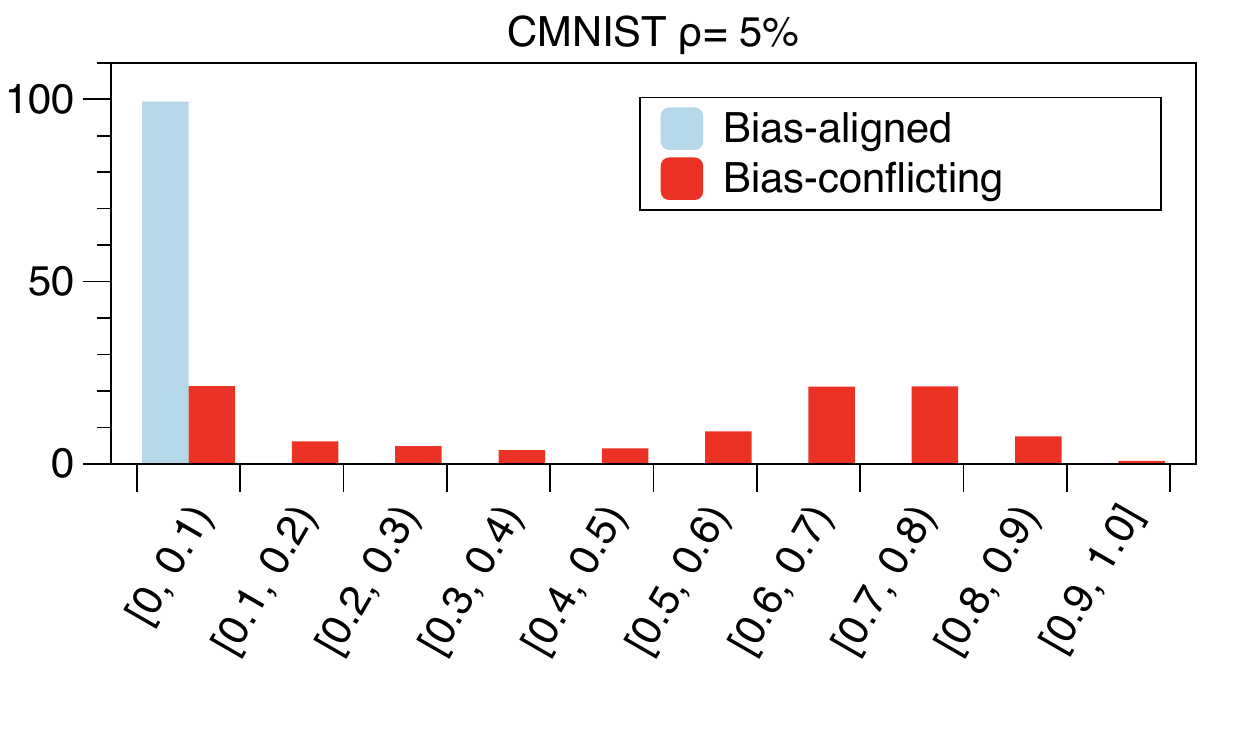} \label{fig:hist_5}}
    \caption{Histogram of per-sample gradient norm.}
    \label{fig:ab_hist}
\end{figure*}

\revision{\subsubsection{Histogram of per-sample gradient norm} To check if the per-sample gradient norm efficiently separates the bias-conflicting samples from the bias-aligned samples, we plot the gradient norm distributions of the colored MNIST. For comparison, we normalized the per-sample gradient norm as follows: $\frac{\norm{\nabla_\theta \mc{L}_{\text{CE}}(x_i,y_i;\theta_b)}}{\max_{(x_i,y_i) \in \mc{D}_n} \norm{\nabla_\theta \mc{L}_{\text{CE}}(x_i,y_i;\theta_{b})}}$. As in Figure~\ref{fig:ab_hist}, the bias-aligned sample has a lower gradient norm (blue bars) than the bias-conflicting samples (red bars). }

% We plot the gradient norm distribution of the bias-conflicting samples and the bias-aligned samples to determine whether the per-sample gradient norm distinguishes them effectively. The reported value is normalized to the maximum value for comparison purposes: \emph{i.e.,} $\frac{\norm{\nabla_\theta \mc{L}_{\text{CE}}(x_i,y_i;\theta_b)}}{\max_{(x_i,y_i) \in \mc{D}_n} \norm{\nabla_\theta \mc{L}_{\text{CE}}(x_i,y_i;\theta_{b})}}$. As shown in Figure~\ref{fig:ab_hist}, the bias-conflicting sample has a higher gradient norm than the aligned sample. In conclusion, we can affirm that the gradient norm has sufficient sample discrimination ability.}
% To determine whether the per-sample gradient norm distinguishes the bias-conflicting samples well, we plot the gradient norm distribution of the bias-conflicting sample and the bias-aligned sample. Report the value scaled to the maximum value for easy comparison: \emph{i.e.,} $\frac{\norm{\nabla_\theta \mc{L}_{\text{CE}}(x_i,y_i;\theta_b)}}{\max_{(x_i,y_i) \in \mc{D}_n} \norm{\nabla_\theta \mc{L}_{\text{CE}}(x_i,y_i;\theta_{b})}}$. As in Figure~\ref{fig:ab_hist}, we can see that the bias-conflicting sample has a larger gradient norm than the aligned samples. In conclusion, we can confirm that the gradient norm has sufficient discriminating bias-conflicting sample ability.}

\begin{wraptable}[6]{r}{0.5\textwidth}
    \vspace{0.5in}
    \centering
    \resizebox{0.5\textwidth}{!}{
    \begin{tabular}{ccccc}
            \thickhline
                                    & Vanilla & LfF & Disen & ours \\ \hline
            Computation time        & 14m 59s  & 21m 35s   & 23m 18s & 33m 31s \\ \thickhline
                                    & Step 1 & Step 2 & Step 3  &\\ \hline
            Computation time        & 15m 19s  & 1m 26s   & 16m 46s &   \\ \thickhline
            
    \end{tabular}
    }
    \caption{Computation cost}
    \label{tab:compute_time}
\end{wraptable}

\revision{\subsubsection{Computation cost} Debiasing requires more modules, which increases the computational cost. The training time for the colosed MNIST $\rho=0.5\%$ is reported in Table~\ref{tab:compute_time}. As in the top of Table~\ref{tab:compute_time}, we report the computational cost of four algorithms, vanilla, LfF, Disen, and PGD. Here, PGD spends a longer training time. To check which parts generate longer time, we measure part-by-part cost, at the bottom of Table~\ref{tab:compute_time}. Note that Steps 1, 2, and 3 represent training the biased model, computing per-sample gradient norm, and training the debiased model, respectively. We can conclude the following two facts. (1) Step 2 (computing per-sample gradient norm) spends $4.3\%$ of training time. (2) Resampling requires an additional cost of 1 m 27s.}

\begin{wraptable}[6]{r}{0.5\textwidth}
    \vspace{0.5in}
    \centering
    \resizebox{0.5\textwidth}{!}{
    \begin{tabular}{ccccc}
            \thickhline
                            & \multicolumn{2}{c}{Training time}        & \multicolumn{2}{c}{Test Acc.}        \\
            Colored MNIST    & Single-stage    & Multi-stage        & Single-stage & Multi-stage\\ \hline
            $\rho=0.5\%$        & 2h 53m 40s  & 33m 39s   & 92.39  & 96.88    \\ 
            $\rho=1\%$        & 2h 54m 45s  & 32m 28s   & 97.10  & 97.35    \\ 
            $\rho=5\%$        & 2h 49m 31s  & 34m 13s   & 98.51  & 98.62    \\ 
            \thickhline
    \end{tabular}
    }
    \caption{Multi-stage versus Single-stage}
    \label{tab:single_stage}
\end{wraptable}

\revision{\subsubsection{Multi-stage vs Single-stage} PGD computes per-sample gradient only once, between training the biased model and the debiased model. However, an update of the per-sample gradient can be performed repeatedly at each epoch (\emph{i.e.,} Single-stage). In other words, the PGD can be modeled to run the following loop: updating the biased model $\to$ updating the sampling probability $\to$ updating the debiased model. In this section, we justify why we compute per-sample gradient at once (\emph{i.e.,} Multi-stage). We report the performance of Multi-stage and Single-stage of PGD on the colored MNIST dataset. As in Table~\ref{tab:single_stage}, the single-stage method has two characteristics: (1) It takes a long training time compared to the multi-stage method. (2) It has lower unbiased test accuracy compared to the multi-stage method. The reason why it takes longer training time is that computing the per-sample gradient norm requires huge computation resources. On the other hand, the sampling probability of the single-stage method changes training distribution over epochs, the debiased model suffers unstable training, so that it loses the debiasing performance.  }
% Our algorithm takes a multi-stage learning method with separate learning for step 1 (biased model training) and step 3 (debiased model training). To justify the learning style of our multi-stage model, we compare the results on the colored MNIST with those of single-stage PGD, which performs gradient norm-based learning by computing the gradient just before each epoch. There are a total of two analyses of single-stage PGD. (1) training time; and (2) training results (unbiased test accuracy).  As in Table~\ref{tab:single_stage}, single stage spends almost $\times 4.7 $ times more than the multi-stage, while the performance is worse. It can be inferred that changing the sampling probability every before the start of each epoch adds a lot of extra computations and also hinders the debiased model from being stable because of the distribution shift. }

\begin{wraptable}[4]{r}{0.4\textwidth}
    \vspace{0.5in}
    \centering
    \resizebox{0.4\textwidth}{!}{
    \begin{tabular}{ccc}
            \thickhline
                            
            Colored MNIST    & Resampling    & Reweighting\\ \hline
            $\rho=0.5\%$        & 96.88  & 94.70 \\ 
            $\rho=1\%$        & 97.35  & 97.20 \\ 
            $\rho=5\%$        & 98.62  & 98.51 \\ 
            \thickhline
    \end{tabular}
    }
    \caption{Reweighting versus resampling}
    \label{tab:reweighting}
\end{wraptable}
        
\revision{\subsubsection{Resampling versus Reweighting} We provide further experimental analysis, \emph{i.e.,} resampling versus reweighting, to support our algorithm design. Reweighting~\cite{nam2020learning, lee2021learning} and resampling~\cite{liu2021just} are the two main techniques to debias by up-weighting bias-conflicting samples. PGD is an algorithm that modifies the sampling probability by using the per-samplge gradient norm. To check whether PGD works with reweighting, we examine the results of PGD with reweighting on colored MNIST datasets and report in Table~\ref{tab:reweighting}. We compute the weight for each sample as follows: $w(x_i,y_i) = |\mc{D}_n| \times \frac{\norm{\nabla_\theta \mc{L}_{\text{CE}}(x_i,y_i;\theta_b)}}{\sum_{(x_i,y_i) \in \mc{D}_n} \norm{\nabla_\theta \mc{L}_{\text{CE}}(x_i,y_i;\theta_{b})}}$. As in Table~\ref{tab:reweighting}, PGD with resampling slightly outperforms PGD with reweighting. As argued in~\cite{an2020resampling}, his gain from resampling can be understood by the arguments that resampling is more stable and better than reweighting. }

\begin{wraptable}[9]{r}{0.45\textwidth}
    \vspace{0.45in}
    \centering
    \resizebox{0.45\textwidth}{!}{
    \begin{tabular}{ccccc}
            \thickhline
            Colored MNIST    & $\alpha=0.3$    & $\alpha=0.5$ & $\alpha=0.7$ & $\alpha=0.9$\\ \hline
            \multicolumn{5}{c}{Debiased model}                \\ \hline
            $\rho=0.5\%$        & 89.93  & 94.70 & 96.88 & 96.79 \\ 
            $\rho=1\%$          & 96.32 & 97.27 & 97.35 & 97.59 \\ 
            $\rho=5\%$          & 98.80 & 98.82 & 98.62 & 98.78 \\ \hline
            \multicolumn{5}{c}{Biased model}                \\ \hline
            $\rho=0.5\%$        & 19.86  & 18.70 & 18.12 & 17.39 \\ 
            $\rho=1\%$          & 22.40 & 21.04 & 19.71 & 19.12 \\ 
            $\rho=5\%$          & 53.24 & 49.46 & 43.97 & 39.40 \\ \hline
            \thickhline
    \end{tabular}
    }
    \caption{Ablation study on GCE parameter $\alpha$.}
    \label{tab:gce_ablation}
\end{wraptable}
        
\revision{\subsubsection{Ablation study on GCE parameter $\alpha$} The only hyper-parameter used specifically in PGD is the GCE parameter $\alpha$. We experimented with this value at $0.7$ according to the protocoal of LfF~\cite{nam2020learning}. However, we need to compare the various cases $\alpha$ on the colored MNIST benchmark for analysis. As in Table~\ref{tab:gce_ablation}, when the GCE parameter is $0.9$, the debiased model performs best. This is because the biased model is fully focused on the bias feature, rather than seeing the target feature, which can be seen from the unbiased test accuracy of the biased model (see the bottom of Table~\ref{tab:gce_ablation}). }

\begin{wraptable}[8]{r}{0.25\textwidth}
    \vspace{0.45in}
    \centering
    \resizebox{0.25\textwidth}{!}{
    \begin{tabular}{cccc}
            \thickhline
            Vanilla    & LfF & Disen & Ours \\ \hline
            \multicolumn{4}{c}{$\rho=90\%$ Colored MNIST}                \\ \hline
            99.04 & 98.75 & 99.31 & 98.43 \\  \hline
            \multicolumn{4}{c}{Natrual CIFAR10}                \\ \hline
            94.24  & - & - & 94.79 \\ 
            \thickhline
    \end{tabular}
    }
    \caption{Results on unbiased colored MNIST and natural CIFAR10 cases.}
    \label{tab:natural}
\end{wraptable}

\revision{\subsubsection{PGD on unbiased datasets} Since PGD changes the given training distribution, it is necessary to check whether the training performance of PGD is degraded or not. To verify this, we report two types of additional results: (1) unbiased colored MNIST ($\rho = 90\%$), and (2) conventional public datasets, \emph{i.e.,} CIFAR 10. We follow experimental settings of colored MNIST for the unbiased colored MNIST. On the other hand, we train ResNet18~\cite{he2016deep} for CIFAR 10 with the SGD optimizer, $0.9$ momentum, $5e-4$ weight decay, $0.1$ learning rate, CosineAnnealing LR decay scheduler. As in Table~\ref{tab:natural}, PGD does not suffer a significant performance degradation in unbiased Colored MNIST. Furthermore, it performs better than the vanilla model on the CIFAR 10 dataset. This means that the training distribution that PGD changes does not cause significant performance degradation. In other words, PGD can only balance the training data set, regardless of whether the training dataset is balanced or unbalanced.}

% Since PGD changes the training distribution, it is necessary to consider the concern that training performance is degraded. To confirm this, we report two types of experimental results: (1) unbiased colored MNIST ($\rho=90\%$), and (2) natural CIFAR10. We used SGD optimizer, ResNet18 model, and cosine annealing scheduler, learning rate 0.1, weight decay 5e-4, and momentum 0.9 to train the CIFAR10 case.  As in Table~\ref{tab:natural}, PGD suffers some performance degradation in the unbiased colored MNIST case, while it obtains better performance for the natural CIFAR10 case. This means that the training distribution that PGD changes does not cause significant performance degradation.}

\begin{wraptable}[6]{r}{0.35\textwidth}
    \vspace{0.45in}
    \centering
    \resizebox{0.35\textwidth}{!}{
    \begin{tabular}{c|cc|cc}
            \thickhline
                Alg.  & \multicolumn{2}{c}{Vanilla} & \multicolumn{2}{c}{Ours} \\ \hline
                Target & Digit & Color & Digit & Color \\ \hline
            $\rho=0.5\%$& 60.94 & 90.33 & 96.88 & 98.92 \\ 
            $\rho=1\%$& 79.13 & 92.53 & 98.35 & 99.58 \\ 
            $\rho=5\%$& 95.12 & 96.96 & 98.62 & 99.70 \\ 
            \thickhline
    \end{tabular}
    }
    \caption{Reverse colored MNIST}
    \label{tab:reverse}
\end{wraptable}

\revision{\subsubsection{Reverse Colored MNIST case} Recent work~\cite{zhang2022rich} argue that prior debiasing algorithms mainly target to learn the second-easiest representation, regardless of the target feature. We report an experimental analysis of what happens if the target becomes a color and the bias feature becomes a digit shape. To verify it, the experiment was conducted by changing only the target and bias feature in the setting of a colored MNIST. As in Table~\ref{tab:reverse}, the performance of the vanilla model does not decrease significantly. This can be empirically proven to show that color is the easier-to-learn feature than the digit shape, as argued in LfF~\cite{nam2020learning}. In addition, as in the PGD results, it is not affected whether the bias attribute is easier to learn than the target attribute. In other words, empirically, PGD does not learn only the second-easiest feature.}

\newpage

\begin{wraptable}[6]{r}{0.2\textwidth}
    \vspace{0.4in}
    \centering
    \resizebox{0.2\textwidth}{!}{
    \begin{tabular}{c|cc}
            \thickhline
                Alg.  & Avg. & Worst \\ \hline
                
            Vanilla$^\dagger$& 92.1 & 58.6  \\ 
            LfF$^\dagger$& 92.5 & 58.8  \\ 
            EIIL$^\dagger$& 90.5 & 67.0  \\ 
            JTT$^\dagger$& 91.1 & 69.3  \\ 
            CnC$^\dagger$& 81.7 & 68.9  \\ 
            Ours$^\dagger$& 92.1 & 70.6  \\ 
            \thickhline
    \end{tabular}
    }
    \caption{CivilComment}
    \label{tab:nlp}
\end{wraptable}

\revision{\subsubsection{Real-world NLP task, CivilComments} In order to observe that does PGD works on another task, such as NLP, and much more realistic case, we test PGD on CivilComments dataset from WILDs benchmarks~\cite{koh2021wilds}. We follow the experimental setting of~\cite{liu2021just}. The $\dagger$ mark represents the reported value in~\cite{zhang2022correct}. As in Table~\ref{tab:nlp}, PGD outperforms the other benchmarks. Therefore, we can conclude that PGD works in another type of network, a transformer, and it is applicable to the real-world. }

% \begin{wraptable}[6]{r}{0.3\textwidth}
%     \centering
%     \resizebox{0.3\textwidth}{!}{
%     \begin{tabular}{ccc}
%             \thickhline
%             Waterbird       & Avg    & Worst   \\ \hline
%             ERM$^*$         & $97.30$  & $72.60$    \\ \hline
%             JTT$^*$         & $93.30$  & $86.70$ \\ \hline
%             Ours            & $96.73$  & \textbf{$88.91$} \\ 
%             \thickhline
%     \end{tabular}
%     }
% \end{wraptable}

% \subsection{Additional dataset, Waterbird}
% We provide experimental comparisons in an additional dataset, Waterbird. The target attribute is to distinguish between two bird sets. One set is the collection of birds living in the water, and the other set is the collection of birds living in the forest. The bias attribute is the background of the data. In other words, an example of a bias-aligned sample is a bird living on the water, a water background, and an example of a bias-conflicting sample is a bird living on the water, a forest background. This experiment is the same as the experimental environment of the JTT paper~\cite{liu2021just} and $*$ mark denotes reported performance in~\cite{liu2021just}.
